# Supplementary material for: Realization of independent contacts in barrier-separated InAs/GaSb quantum wells
Source: arXiv:2303.06621 source file (2023-03-12)
Supplement: Supplementary file 1 [file Supplementary_Material.pdf]

# Realization of independent contacts in barrier-separated InAs/GaSb quantum wells

Xingjun Wu,<sup>1, a)</sup> Jianhuan Wang,<sup>1</sup> Miaoling Huang,<sup>1</sup> Shili Yan,<sup>1</sup> and Rui-Rui Du<sup>2, a)</sup>

<sup>1)</sup>Beijing Academy of Quantum Information Sciences, Beijing, 100193, China

<sup>2)</sup>International Center for Quantum Materials, School of Physics, Peking University, Beijing 100871, China

## I. THE BASIC MATERIAL QUALITY METRICS ABOUT THE SAMPLE

The cross-sectional high-resolution TEM micrograph of the material along the (011) direction is shown in Fig. S1(a). It can be found that the crystalline structure remains coherent across each quantum well interface. Moreover, the TEM analysis shows that the top and bottom interface root-mean-square (RMS) roughness of InAs QW are around 2.4 Å and 2.2 Å, respectively. The sample surface morphology is also characterized by AFM as shown in Fig. S1(b). The RMS surface roughness of the sample achieves around 1.2 Å over an area of  $1 \mu\text{m} \times 1 \mu\text{m}$ .

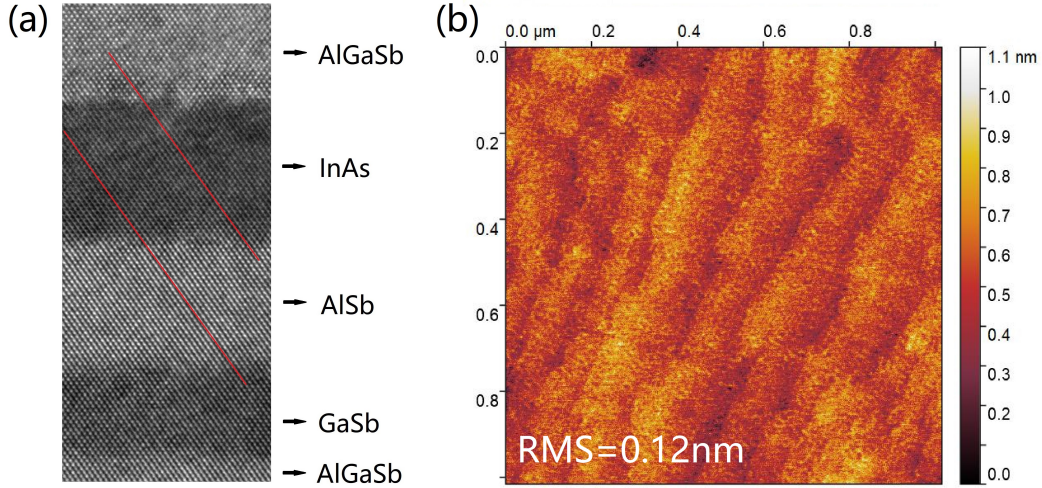

FIG. S1. (a) High-resolution TEM micrograph of the InAs/GaSb QWs. (b) AFM image of the InAs/GaSb sample surface.

In addition, we have used geometric phase analysis (GPA) to map strain distribution from the cross-sectional high-resolution TEM image in Fig. S2 (a), and the strain component maps along the horizontal ( $\epsilon_{xx}$ ) and the vertical axis ( $\epsilon_{zz}$ ) are shown in Fig. S2(b) and S2(c), respectively. Here, the top AlGaSb layer is considered strain-relaxed. We find that the mapping of  $\epsilon_{xx}$  in the whole structure is homogeneous and close to zero. This finding indicates that the in-plane arrangement of InAs follows the underlying AlSb lattice, resulting in the biaxial tensile strain. Due to strain relaxation, the out-of-plane strain of the InAs QW theoretically should be in compression, which is consistent with our observation in Fig. S2(c). The same analysis can be applied to GaSb QW.

## II. MAGNETORESISTANCE OSCILLATION OF THE 2DHG AT A FIXED MAGNETIC FIELD

The hole density is estimated by sweeping back gate bias at a fixed magnetic field. To characterize the hole density, we prepared a dual-gated Hall-bar device of  $60 \mu\text{m} \times 20 \mu\text{m}$  size, of which the front gate was fabricated by evaporating Al from the front side, while the back gate was fabricated by evaporating Al from the opposite with a "flip-chip" process<sup>1</sup>. The processing

<sup>a)</sup> Authors to whom correspondence should be addressed: [Xingjun Wu, wuxj@baqis.ac.cn; Rui-Rui Du, rrd@rice.edu]

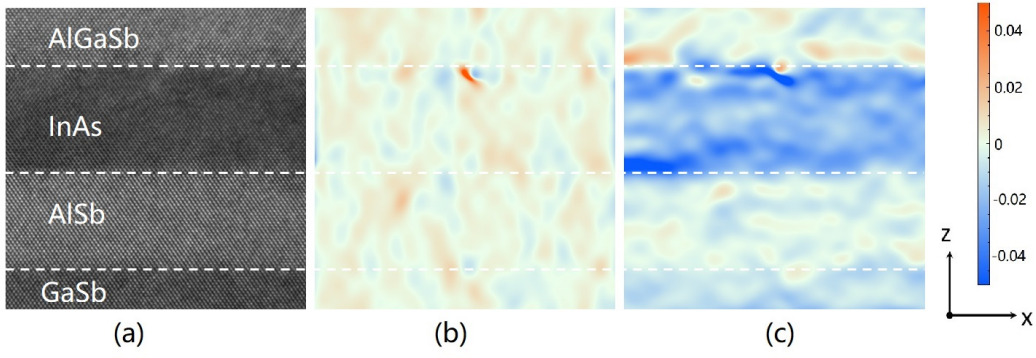

FIG. S2. Strain distribution map along (b) the horizontal axis  $\epsilon_{xx}$  and (c) the vertical axis  $\epsilon_{zz}$ , after applying GPA to the region displayed in (a).

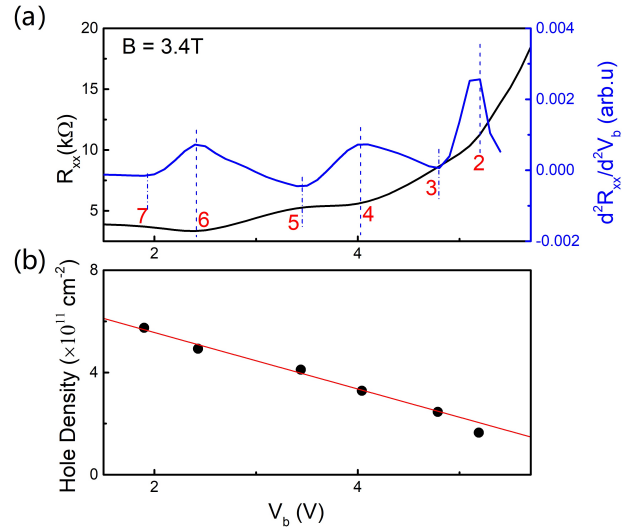

FIG. S3. (a) Magnetoresistance oscillation of the 2DHG by sweeping back gate voltage at  $B = 3.4$  T. The second derivative of the resistance are plotted with the blue curve. (b) The back gate voltage dependence of the hole density.

details can be found in our other study<sup>2</sup>. In the device, we apply a negative bias to the front gate (e.g.,  $V_f = -1.13$  V in this case,  $n \sim 0.4 \times 10^{11} \text{ cm}^{-2}$ ) to increase the resistance in the electron layer, which facilitates the observation of the magnetoresistance oscillation of the holes. Fig. S3(a) shows the back gate voltage-dependent longitudinal resistance at  $B = 3.4$  T. We find that, as the back gate is biased positively, the hole density decreases, and the longitudinal resistance increases. At the same time, due to the formation of the Landau level in the magnetic field, the longitudinal resistance shows a periodic oscillation behavior. The second derivative of the resistance was used in Fig. S3(a) to analyze the extrema. Since the Zeeman splitting in GaSb QW is much smaller than the Landau level spacing (g-factor  $\sim 0.9^3$ ), the resistance minima at the odd filling factors caused by Zeeman splitting would be difficult to detect in oscillation, especially if the hole mobility is not high. Therefore, the periodic emergence of resistance minima in the sweeping should correspond to a set of states with even filling factors in the Landau levels.

In addition, we find that when the back gate voltage  $V_b > 4.5$  V, the resistance begins to increase rapidly. The voltage around 5.1 V is the maximum gate bias at which the resistance minima can be observed experimentally. Based on the upward trend of the curve, the resistance at the next expected minimum would be quite large despite the parallel effect of the electron gas, which can be considered as the case of almost depletion of the hole. Therefore, it is reasonable to speculate that the resistance minimum at  $V_b = 5.1$  V corresponds to the state with the filling factor of 2. With the decrease of the gate bias, the hole density increases, and the Fermi level successively passes through the Landau levels of filling factors 4 and 6, resulting in the corresponding occurrence of the resistance minima. The back gate voltage dependence of the hole density is plotted in Fig. S3(b). Good linearity verifies

the periodicity of the resistance oscillations. The line slope indicates the modulation of the back gate potential to the hole density is about  $1 \times 10^{11} \text{ cm}^{-2}/\text{V}$ , which is consistent with the results estimated from the plane capacitor model. According to the linear relation, we infer that the hole density at  $V_b = 0 \text{ V}$  is about  $7.7 \times 10^{11} \text{ cm}^{-2}$ .

The hole mobility is estimated by the longitudinal resistivity expression at zero magnetic fields using the two-carrier model,  $\rho_{xx} = 1/e(n\mu_e + p\mu_h)$ , where the electron mobility ( $\mu_e \sim 1 \times 10^5 \text{ cm}^2\text{V}^{-1}\text{s}^{-1}$ ) is extracted from the InAs single layer transport in Fig. 2(c). Using the calculated electron and hole densities, we thus arrive at the hole mobility ( $\mu_h \sim 1 \times 10^4 \text{ cm}^2\text{V}^{-1}\text{s}^{-1}$ ).

### III. INTERLAYER NONLINEARITY

For the device shown in Fig. 3(c), the current-voltage curves under different measurement circuits are plotted in Fig. S4, where the insets represent the corresponding electrical measurement circuits. We find that the  $I-V$  curves are linear when the drive current is limited to the single-layer section of the electrical circuits. The nonlinear characteristic only appears when the drive current crosses the InAs/AlSb/GaSb junction interface, indicating the nonlinear behavior is related to the junction. In addition, the different slopes of the  $I-V$  curve in Fig. S4(a) and S4(b) are attributed to imperfect interlayer isolation. The current flowing through one layer would create a shunt between the two layers, hence different slopes.

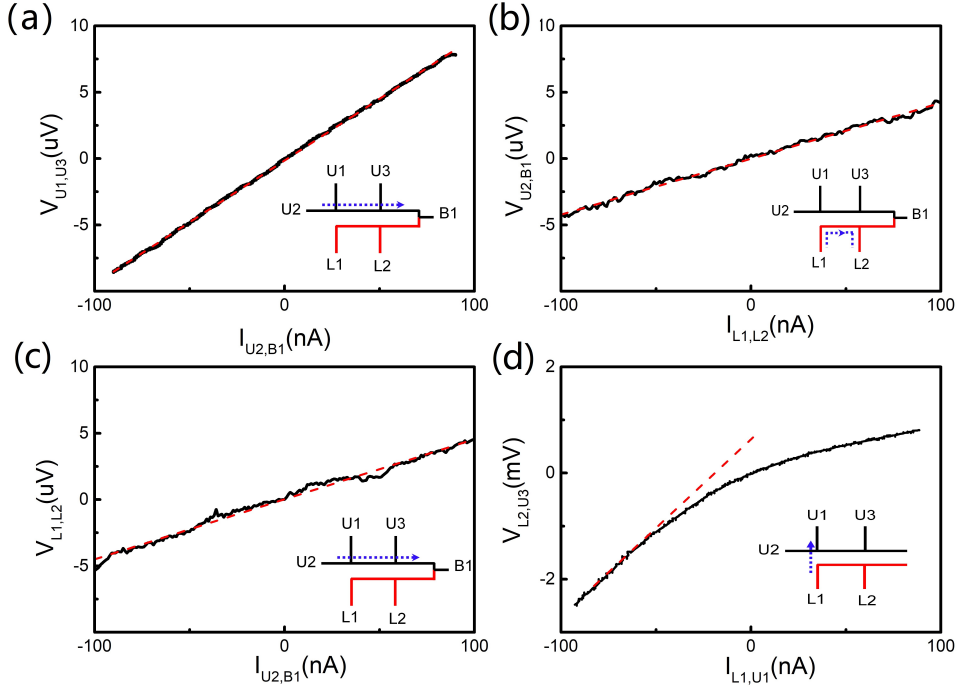

FIG. S4. The current-voltage curves for different electrical measurement circuits. The insets show the corresponding sketch of the device in Fig. 3c. In particular, the inset of (d) shows that the contact B1 in the device is being cut off and the two layers are separated. Here,  $I_{m,n}$  represents the drive current flowing from the contact m to n, and  $V_{k,t}$  represents the voltage drop measured between the contact k and t.

<sup>1</sup>M. Weckwerth, J. Simmons, N. Harff, M. Sherwin, M. Blount, W. Baca, and H. Chui, *Superlattices and Microstructures* **20**, 561 (1996).

<sup>2</sup>X.-J. Wu, W. Lou, K. Chang, G. Sullivan, A. Ikhlassi, and R.-R. Du, *Physical Review B* **100**, 165309 (2019).

<sup>3</sup>X. Mu, G. Sullivan, and R.-R. Du, *Applied Physics Letters* **108**, 012101 (2016).
